# Supplementary material for: Dynamic Prompting: A Unified Framework for Prompt Tuning
Source: arXiv:2303.02909 source file (2023-05-27)
Supplement: Supplementary file 1 [file s8_appendix.tex]

\newpage
\section*{\centering \Large{Appendix: DNA-GPT}}

\section*{Limitations and Broader Impact}
Our proposed method, \methodname, is specifically designed to detect GPT-generated text produced by AI models like ChatGPT. However, we must emphasize that our current evaluation has been limited to language models resembling the GPT decoder-only architecture. We do not claim that our method can reliably detect text generated by non-decoder-only models.
Furthermore, our method is only tested for detecting text within a moderate length range(1000-2000 characters). Texts significantly shorter or longer than what we have tested may not yield accurate results.
It is crucial to acknowledge that our method might still make mistakes. Users should exercise caution and assume their own risk when utilizing our detector. Finally, it is essential to clarify that the detection results do not necessarily reflect the views of the authors.

\section{Theoretical Analysis}\label{app:theory}

\subsection{Is it always possible to distinguish between AI-generated text and Human?}
The recent work exploits the possibility of AI-generated text by analyzing the \texttt{AUROC} for any detector $D$. Armed with the LeCam's lemma \citep{le2012asymptotic,wasserman2013} which states that for any distributions $M$ and $H$, given an observation $s$, the minimum sum of Type-I and Type-II error probabilities in testing whether $s \sim M$ versus $s \sim H$ is equal to $1 {-} \texttt{TV} (M, H)$. Here, \texttt{TV} denotes the total variance between two distributions. %\todoq{add a definition of TV}
Hence, this can be interpreted as :
\begin{align}\label{ROC_upper}
    \text{TPR}_{\gamma} \leq \min\{\text{FPR}_{\gamma} + \texttt{TV}(M, H),1\},
\end{align}

where $\text{TPR}_{\gamma}\in[0,1]$. The upper bound in \eqref{ROC_upper} is leveraged in one of the recent work \citep{sadasivan2023can} to derive \texttt{AUROC} upper bound $\texttt{AUC} \leq \frac{1}{2} + \texttt{TV} (M, H) - \frac{\texttt{TV} (M, H)^2}{2}$ which holds for any $D$. 
This upper bound led to the claim of impossibility results for reliable detection of AI-Generated Text when $\texttt{TV} (M, H)$ is approaching 0. The upper bound in \eqref{ROC_upper} is also interpreted as either certain people’s writing will be detected falsely as AI-generated or the AI-generated text will not be detected reliably when $\texttt{TV} (M, H)$ is small. However, another work \cite{chakraborty2023possibilities} derives an opposite conclusion. Based on the large deviation theory in \cite[Chapter 7]{polyanskiy2022information}, Proposition 3.1 \cite{chakraborty2023possibilities} proves that the upper bound of AUROC increases exponentially with respect to the number of samples n. This means that even if the machine and human distributions were close in the sentence space, by collecting more sentences, it is possible to inflate the total variation norm to make the detection possible. Despite those results, we provide additional analysis, as illustrated in the next section.
\subsection{On the pursuit of TPR and FPR.}
First, we argue that AUROC is not a perfect indicator since it is clear that an AUROC score of 0.99 could lead to 0\% TPR under 1\% FPR. Drawn from the conclusion in \cite[Chapter 14.5]{polyanskiy2022information}, it is shown that if we allow the type-I error to be 0.999, it is impossible for the type-II error to decay faster. This means that despite the conclusion in \cite{chakraborty2023possibilities} that AUROC increases exponentially with respect to the number of samples n, there is still some fundamental difficulty in obtaining both good type-I and II errors. 

Stein's lemma \cite[Theorem 14.13]{polyanskiy2022information} states that for an FPR < 0.001, if we want to pursue $TPR > 1 {-} 10^{{-}40} $, then a rule of thumb for the required sample size is:
$$n \geq - \frac{log 10^{-40}}{D(M||H)}, $$
 where $D(M||H)$ is the KL divergence between the two distributions.

% 1 - α (<=ϵ) is a false positive
% 1 - β is known as a true positive

% \textbf{Gaussian Mixture model} 
% Suppose the human distribution $H$ is composed of many individual human distributions $\{h_1, ..., h_N  \}$. We claim that even if $\texttt{TV} (M, H) = 0$, $\texttt{TV} (M(S_1|S_2), h_i(S_1|S_2)) \neq 0$ always holds.

% Chernoff Bound:
% suppose $X=\sum_{i=1}^n X_i$, $X_1$, $X_2$, $...$, $X_n$ are iid. poisson experiments, $\mu=E[X]$

% 1. For $0 < \delta \leq 1 $

% $$Pr[X\ge (1+\delta)\mu] \leq exp\bigg(-\frac{\mu\delta^2}{2} \bigg) $$

% $$Pr[X\le (1-\delta)\mu] \leq exp\bigg(-\frac{\mu\delta^2}{2} \bigg) $$

\newpage
\section{Additional Experimental Results}\label{app:parameter}
\subsection{Prompts and datasets}
We use 200, 200, 150, 200, and 300 instances from Reddit, Scientific
Abstracts, PubMedQA, Xsum, and WikiText, respectively.
The used system and user prompt on different datasets are outlined in Table \ref{tab:prompts} for \texttt{gpt-3.5-turbo} and \texttt{gpt-4-0314}. For other models without the system prompt input, we only use the user prompt.
\begin{table}[htbp]
    \centering
    \caption{Examples of prompts used in different datasets.}
    \newcommand{\systemprompt}{System: You are a helpful assistant that answers the question provided.}
    \newcommand{\userprompt}[1]{User: Answer the following question in #1 words: \textit{Question}}
    \newcolumntype{Y}{>{\centering\arraybackslash}m{1.5cm}}
    \begin{tabularx}{\textwidth}{Y|>{\centering\arraybackslash}X}
        \hline
         \textbf{Datasets} & \textbf{Prompts}  \\
        \hline
        \multirow{2}{=}{Reddit} & \systemprompt \\ \cline{2-2}
        & \userprompt{180-300} \\
        \hline
        \multirow{2}{=}{Scientific Abstracts} & System: You are a research scientist. Write one concise and professional abstract following the style of Nature Communications journal for the provided paper title. \\ \cline{2-2}
        & User: Title: \textit{title} \\
        \hline                  
        \multirow{2}{=}{PubMedQA} & \systemprompt \\ \cline{2-2}
        & User: \textit{Question} \\
        \hline
        \multirow{2}{=}{Xsum} & System: You are a helpful assistant that continues the sentences provided. \\ \cline{2-2}
        & User: Complete the following sentences for a total of around 250 words: \textit{Prefix} \\ 
         \hline
        \multirow{2}{=}{WikiText} & System: You are a helpful assistant that continues the sentences provided. \\ \cline{2-2}
        & User: Complete the following sentences for a total of around 250 words: \textit{Prefix} \\ 
        \hline
    \end{tabularx}
    \label{tab:prompts}
\end{table}

\subsection{Model memorization}
As mentioned in Section \ref{sec:Memorization}, the model has the potential to retain training data, resulting in the generation of verbatim copying text. To illustrate this point, we conducted an experiment using WikiText-103. 
\sloppy
\begin{wraptable}{l}{0.55\textwidth}
\centering
\caption{Overall comparison of different methods on WikiText-103 datasets. The TPR is calculated at 1\% FPR.
}\label{tab:wikitext} 
% \resizebox{0.96\textwidth}{!}
% {
\begin{tabular}{lcc}
\toprule
\quad \quad\quad\quad Dataset$\rightarrow$ & \multicolumn{2}{c}{WikiText-103} \\% Mixed-all
\cmidrule(lr){2-3} 
Methods$\downarrow$ & AUROC & TPR  \\
\midrule
%%%%%%%%% GPT-4-0314
\multicolumn{3}{c}{\done  \texttt{GPT-4-0314(Black-box)} }\\
\midrule
GPTZero & \textbf{92.00} & 0.00  \\
OpenAI& 82.45 & \textbf{32.67}  \\
\midrule
\methodname~, $K$=5, $\gamma$=0.7 & 90.77 & 0.33  \\
% \qquad $K$=10, $\gamma$=0.5 & - & -  \\
\midrule
\multicolumn{3}{c}{\done  \texttt{GPT-3.5-turbo(Black-box)}} \\
\midrule

%%%%%%%%% GPT-3.5
GPTZero \cite{GPTZero} & 92.67 & 0.33  \\
OpenAI \cite{AITextClassifier} & 93.45 & 55.33  \\
\midrule
\methodname~, $K$=20, $\gamma$=0.7& \textbf{99.63} & \textbf{93.00}  \\
% \qquad $K$=20, $\gamma$=0.5 & - & -  \\

\midrule
\multicolumn{3}{c}{ \done \texttt{text-davinci-003(Black-box)} } \\
\midrule
GPTZero & 92.67 & 0.33  \\
OpenAI & 95.39 & \textbf{72.00}  \\ \hline
\methodname~, $K$=20, $\gamma$=0.7 & 94.40 & 7.00  \\
% \qquad $K$=10, $\gamma$=0.5 & - & -  \\ \\

\midrule
\multicolumn{3}{c}{\doneWhite \texttt{text-davinci-003(White-box)} } \\
\midrule
\methodname~, $K$=20, $\gamma$=0.7 & \textbf{96.67} & 0.67  \\
% \qquad $K$=10, $\gamma$=0.5, & - & -  \\ \\

\bottomrule
\end{tabular}
% }
%\vspace{2.5mm}
\vspace{-0.2cm}
\end{wraptable}

We provided the model with the first 30 words and requested it to continue writing. The two examples of verbatim copies of the generated passages are presented in Table \ref{tab:wiki-copy}. It is clear that a large portion of text pieces are exactly the same as in the original data, showing the LLMs indeed remembered the training text and thus produced verbatim copies. We believe it becomes less meaningful to determine whether such text is either GPT-generated or human-written, considering the model actually reproduces the human-written text.
On the other hand, the detection results are illustrated in Table \ref{tab:wikitext}. It is evident that GPTZero exhibits extremely poor performance in terms of TPR across all models. Furthermore, our methods outperform OpenAI's classifier in the AUROC score, but we also encounter low TPR in \texttt{GPT-4-0314} and \texttt{text-davinci-003}. These results highlight the challenges associated with detecting instances where pre-trained language models memorize a substantial portion of the training data, leading to verbatim copying during text generation and rendering human-written and AI-generated text indistinguishable. Therefore, we recommend utilizing the newest datasets for detection tasks to reduce the potential of being memorized by LLMs, especially when their training data is closed.

\begin{table}[htbp]
    \centering
    \caption{ Examples of verbatim copy(highlighted in \textcolor{red}{red}) from training data in GPT-generated text. Examples are taken from WikiText-103 using \texttt{gpt-tubro-35}. }
    \setlength{\extrarowheight}{2pt}
    \begin{tabularx}{\textwidth}{ >{\centering\arraybackslash}p{1.5cm}|>{\centering\arraybackslash}X |>{\centering\arraybackslash}p{1cm} }
        \toprule
         \textbf{Source} & \textbf{ Text} & Misc\\ \hline
        Prefix & Nevertheless, Die Another Day was the highest-grossing James Bond film up to that time unadjusted for inflation. MI6 agent James Bond infiltrates a North Korean military base where Colonel Tan-Sun Moon is illegally trading weapons for African conflict diamonds. &  \\ 
        \hline
        Human-written & After Moon\'s right-hand man Zao is contacted by an unknown source who reveals ... .  \textcolor{blue}{\faCut} \textcolor{blue}{to his current wealth, celebrity, and philanthropy from its assets. ... At his ice palace adjacent to the diamond mine site in Iceland, \textit{ \textcolor{red}{Graves unveils a new orbital mirror satellite, "Icarus", which is able to focus solar energy on a small area and provide year-round sunshine for crop development. }} }\textcolor{blue}{Frost seduces Bond and Jinx infiltrates Graves' command centre, but is captured by Graves and Zao.}  & truncation ratio = 0.7 \\ 
        \hline
        \multirow{4}{=}{GPT-regeneration} 
        & to his sudden wealth. Bond then meets Graves face-to-face, and is convinced that he is connected to the diamonds somehow. Bond follows Graves and his assistant, Miranda Frost, to an ice palace in Iceland where \textit{\textcolor{red}{Graves unveils a new orbital mirror satellite, "Icarus", which is able to focus solar energy on a small area and provide year-round sunshine for crop development.}} Bond discovers that Graves is ... . &  \textit{Overlap 27-grams}  \\  %\cline{2-2}
        \midrule \hline
        Prefix & Upsilon Andromedae b (v Andromedae b, abbreviated Upsilon And b, v And b), formally named Saffar , is an extrasolar planet approximately 44 light-years away from the Sun in the constellation of Andromeda. The planet orbits the solar analog star, Upsilon Andromedae A, approximately every five days. \\ 
        \hline
        Human-written & Discovered in June 1996 by Geoffrey Marcy and R. Paul Butler, it was one of the first hot ....  \textcolor{blue}{\faCut} \textcolor{red}{lanets and their host stars. The process involved public nomination and voting for the new names. In December 2015, the IAU announced the winning name was Saffar }\textcolor{blue}{ for this planet. The winning name was submitted by the Vega Astronomy Club of Morocco and honours the 11th Century astronomer Ibn al-Saffar of Muslim Spain. }  & truncation ratio = 0.7 \\ 
        \hline
        \multirow{4}{=}{GPT-regeneration} 
        & \textit{\textcolor{red}{lanets and their host stars. The process involved public nomination and voting for the new names. In December 2015, the IAU announced the winning name was Saffar}} submitted by the people of Morocco. ... . &  \textit{Overlap 26-grams}  \\ 
        \bottomrule
    \end{tabularx}

    \label{tab:wiki-copy}
\end{table}

\subsection{Different model versions}
Since OpenAI is actively updating the latest ChatGPT model, e.g. \texttt{gpt-3.5-turbo}, one central question remains: does the method still works when the behind model weights have already changed? To answer this question, we conduct experiments using \texttt{gpt-3.5-turbo} for a time interval. 
\sloppy
\begin{wraptable}{l}{0.55\textwidth}
    \caption{Detection results after a time interval considering the models are being actively updated. }
    \begin{tabular}{lcccc}
    \toprule
    \multicolumn{5}{c}{ \texttt{Model Version}} \\
    \midrule
     \quad Model$\rightarrow$ & \multicolumn{2}{c}{GPT-3.5-turbo} & \multicolumn{2}{c}{GPT-4}  \\% Mixed-all
    \cmidrule(lr){2-3} \cmidrule(lr){4-5}
    Date$\downarrow$ & AUROC & TPR & AUROC & TPR  \\
    \midrule
    04/04/2023 & 99.61 & 87.50 & 99.34 & 91.00 \\
    05/14/2023 & 98.70 & 92.00 & 98.98 & 98.00 \\
    \bottomrule
    \end{tabular}

    \label{tab:version}
\end{wraptable}
Typically, we first generate and store the answers on 04/04/2023 and then perform the detection on 04/15/2023 and 05/01/2023. We also tested \texttt{gpt-4} on 14/05/2023, three months since the release of \texttt{gpt-4-0314}, where the outputs are originally generated by the latter on the Reddit dataset and tested on the former model after such a long time interval. This realistic scenario simulates the detection might be conducted a while after the answer has been generated, during which the updated model might make the original detection challenging. The results are presented in Table \ref{tab:version}. We can see that the performance almost maintains.

\subsection{Inverse prompt inference}\label{app:inverse}
For cases where the prompt questions are unknown, we assert that inverse prompt inference can alleviate such scenarios. For example, the questions in the Reddit ELI5 dataset could possibly be inversely inferred by prompting the answer and asking the model for a possible question. We tried with \texttt{gpt-3.5-turbo} and manually checked the inversely inferred prompts for 20 instances and found 14 of them were very similar to the original questions. However, considering our results without golden prompts already achieved substantial performance, we did not conduct further experiments by using inversely obtained prompts. We believe this approach provides a solution for other datasets when the golden prompts are unavailable and leave more exploration for future work.

\subsection{Sliding window}
\label{app:sliding}
For text co-written by humans and machines, despite the revised text discussion in the previous section, we also consider text where the machine first generates some passages, and then humans continue to write the remaining text. Since the original truncation and then re-prompting pipeline will not directly work when the human-written part does not follow the style of GPT-generated content, we think it is possible to apply a sliding window for detection. More specifically, we can first cut the whole passage into several parts and do the detection on each passage. For simplicity, we simulate such scenarios by using only half machine-generated and half human-written text and combining them together, resulting in text starting with AI-written and followed by human-written. Notice that there might be some influence when combining them together, but we believe it is enough for testing our sliding window approach for simplicity. We perform the experiments using \texttt{gpt-3.5-turbo} on Reddit and Xsum datasets by applying a sliding window for detection, and our methods would classify the results into AI-written as long as any text under their window is classified. We use a window size of 2, namely splitting the text into two parts. Notice the two baselines do not accept shorter text under a specific window, and we use their overall classification results.
The results are shown in Figure \ref{fig:prefix_res}. As we can see, our methods still consistently outperform the two baselines, validating the effectiveness of our sliding window strategy for solving long text starting with machine-generated prefixes and followed by human-written continuation.

\begin{figure*}[!t]\vspace{-0.1cm}

  \centering
    \includegraphics[width=0.9\textwidth,height=0.3 \textwidth]{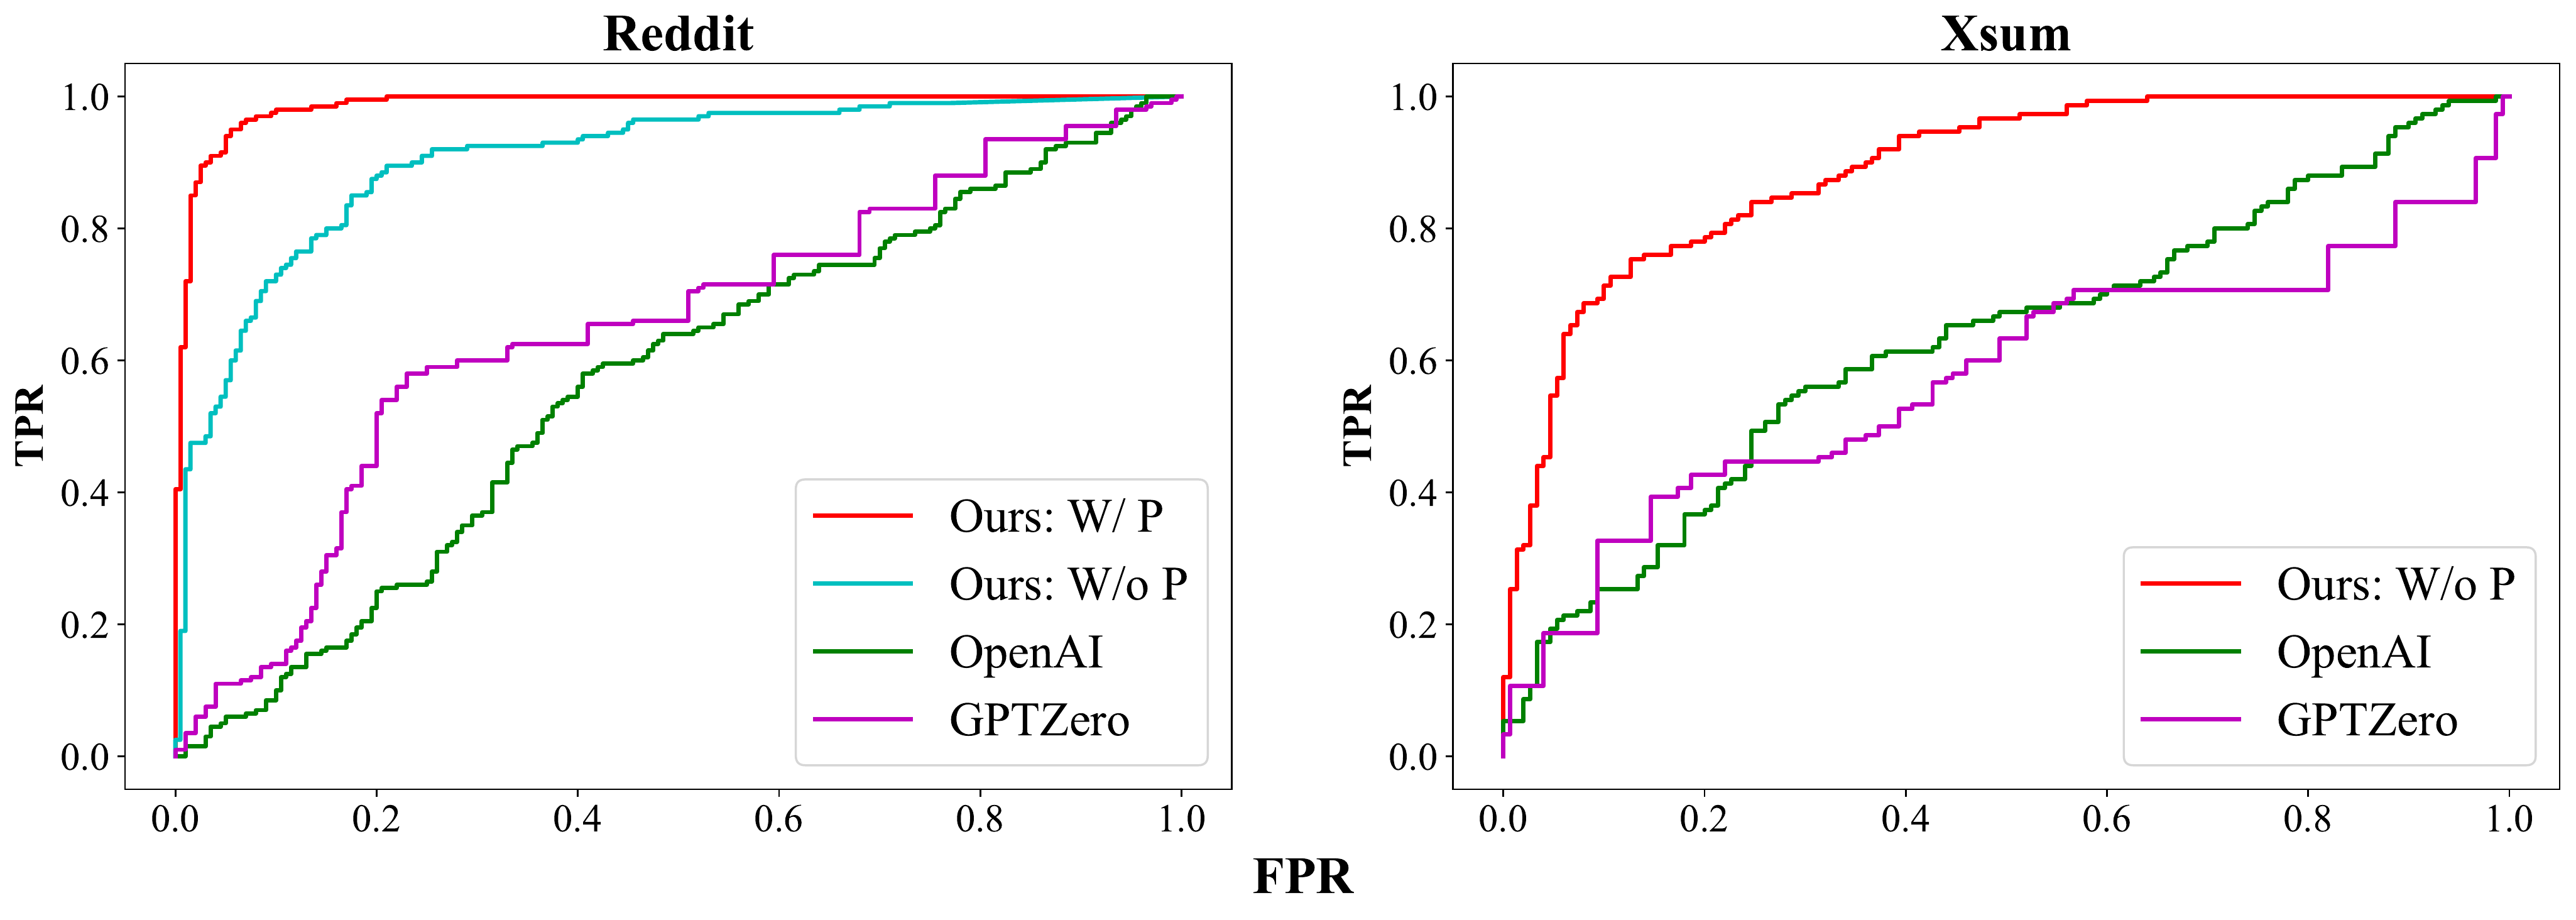}
    \caption{A comparative analysis of the AUROC curve obtained by the sliding window and two baselines. }
    \label{fig:prefix_res}\vspace{-0.5cm}

\end{figure*}

\begin{table}[htbp]
\caption{Parameter sensitivity analysis for choice of the starting $N{-}grams$ $n_0$. Results are reported when the golden prompts are unknown. }
\centering
\resizebox{\textwidth}{!}{%
\begin{tabular}{|c|c|c|c|c|c|c|c|c|c|c|c}
\hline
\quad\multirow{2}{*}{Models$\rightarrow$} & \multicolumn{4}{c|}{\texttt{text-davinci-003}} & \multicolumn{4}{c|}{\texttt{gpt-3.5-turbo}}  \\
\cline{2-9}
 & \multicolumn{4}{c|}{AUROC(TPR)} & \multicolumn{4}{c|}{AUROC(TPR)} \\
\hline
 \textit{$n_0$} & Reddit & PubMedQA & Xsum & Avg.& Reddit & PubMedQA & Xsum & Avg. \\
\hline
\textit{$1$} & 93.55(41.50) &  87.03(24.67) &  97.22(77.00) &  92.60(47.72) & 93.91(47.50) &  93.46(60.00) &  96.87(46.67) &  94.75(51.39)  \\
\textit{$2$} & 92.55(44.00) &  85.72(28.00) &  96.42(77.00) &  91.56(49.67) & 92.74(39.50) &  91.41(55.00) &  95.17(40.67) &  93.11(45.06)  \\
\textit{$3$} & 92.55(44.00) &  85.72(28.00) &  96.42(77.00) &  91.56(\textbf{49.67}) & 92.74(39.50) &  91.41(55.00) &  95.17(40.67) &  93.11(45.06)  \\
\textit{$4$} & 95.42(46.00) &  87.55(22.67) &  96.25(69.00) &  \textbf{93.07}(45.89) & 95.17(49.00) &  95.46(59.00) &  97.45(70.67) &  96.03(\textbf{59.56})  \\
\textit{$5$} & 95.42(46.00) &  87.55(22.67) &  96.25(69.00) &  93.07(45.89) & 95.17(49.00) &  95.46(59.00) &  97.45(70.67) &  96.03(59.56)  \\
\textit{$6$} & 95.93(44.00) &  88.26(22.00) &  95.00(62.00) &  93.06(42.67) & 96.58(54.00) &  95.29(51.00) &  97.08(57.33) &  \textbf{96.32}(54.11)  \\
\hline
\end{tabular}
}
\label{tab:start_gram}
\end{table}

\subsection{Parameter sensitivity analysis}\label{app:sensitivity}
\textbf{Effects of starting and ending N-gram.} The $n_0$ and $N$ in Equation \ref{eq:black} are used to control the overlap ratio measurement of $N{-}grams$. We first set $N$ to $25$ since we find the overlap seldom excels this value and then change $n_0$ to find the best starting value. The results are shown in Table \ref{tab:start_gram}. As we can see, setting $n_0$ to small values or large values like 1 or 6 both hurts performance, and we choose $n_0$ to be $4$ to balance the AUROC and TPR across all models or datasets, as well as provide reasonable explanations.

\textbf{Effects of weight function.} 
The weight function in Equation \ref{eq:black} is primarily used for assigning higher weighting for large overlap of N-grams, while low weights are otherwise. Intuitively, $f(n)$ can be chosen from the simple log function to the exponential function. Hence, we tried the basic functions from $ \{\log(n), n, n\log(n), n\log^2(n), n^2, e^n \}$. The results are shown in Table \ref{tab:function_auroc} and \ref{tab:function_tpr}. Taking both AUROC and TPR into consideration, we report all results using $f(n){=}n\log(n)$.
We admit that our choice might not be optimal, but we stick to it for simplicity.
\begin{table}[htbp]
\caption{Parameter sensitivity analysis for choice of the weighting function. Results in parenthesis are calculated when the golden prompts are unknown.}
\centering
\resizebox{\textwidth}{!}{%
\begin{tabular}{|c|c|c|c|c|c|c|c|c|c|c|c}
\hline
\quad\multirow{2}{*}{Models$\rightarrow$} & \multicolumn{4}{c|}{\texttt{text-davinci-003}} & \multicolumn{4}{c|}{\texttt{gpt-3.5-turbo}}  \\
\cline{2-9}
 & \multicolumn{4}{c|}{AUROC} & \multicolumn{4}{c|}{AUROC} \\
\hline
weight funtion \textit{f(n)$\downarrow$} & Reddit & PubMedQA & Xsum & Avg.& Reddit & PubMedQA & Xsum & Avg. \\
\hline
\textit{$\log(n)$} & 96.83(94.33) &  84.10(86.14) &  93.81(87.55) &  91.58(89.34) &  99.37(93.12) &  91.74(93.89) &  94.90(97.22) &  95.34(94.74)  \\
\textit{$n$} &  97.59(94.93) &  84.96(86.93) & 97.02(92.25) &  93.19(91.37) &  99.59(94.39) &  93.73(94.86) &  96.03(97.30) &  96.45(95.52)  \\
\textit{$n\log(n)$} &  98.06(95.42) &  85.93(87.55) &  98.39(96.42) &  94.12(93.13) &  99.67(95.17) &  95.11(95.46) &  96.58(97.45) &  97.12(96.03)   \\
\textit{$n\log^2(n)$} &  98.39(95.78) &  87.00(88.13) &  97.89(96.96) &  94.43(93.62) &  99.72(95.71) &  96.09(95.93) &  96.78(97.50) &  97.53(96.38)   \\
\textit{$n^2$} &  98.43(95.81) &  86.97(89.18) &  97.78(96.84) &  94.39(\textbf{93.94}) &  99.73(95.78) &  96.21(95.96) &  96.87(97.45) &  97.60(96.40)   \\
\textit{$e^n$} &  98.52(96.37) &  92.55(90.67) &  94.87(94.08) &  \textbf{95.31}(93.71) &  99.44(98.21) &  98.77(95.31) &  97.07(95.96) &  \textbf{98.43}(\textbf{96.49})   \\
\hline
\end{tabular}
}
\label{tab:function_auroc}
\end{table}

\begin{table}[htbp]
\caption{Parameter sensitivity analysis for choice of the weighting function. Results are reported when the golden prompts are unknown. }
\centering
\resizebox{\textwidth}{!}{%
\begin{tabular}{|c|c|c|c|c|c|c|c|c|c|c|c}
\hline
\quad\multirow{2}{*}{Models$\rightarrow$} & \multicolumn{4}{c|}{\texttt{text-davinci-003}} & \multicolumn{4}{c|}{\texttt{gpt-3.5-turbo}}  \\
\cline{2-9}
 & \multicolumn{4}{c|}{TPR} & \multicolumn{4}{c|}{TPR} \\
\hline
weight funtion \textit{f(n)$\downarrow$} & Reddit & PubMedQA & Xsum & Avg.& Reddit & PubMedQA & Xsum & Avg. \\
\hline
\textit{$\log(n)$} & 48.00 &  9.33 &  43.00 &  33.44 & 85.50 &  21.33 &  26.67 &  44.50  \\
\textit{$n$} & 48.50 &  9.33 &  69.00 &  42.28 & 90.00 &  27.33 &  10.00 &  42.44  \\
\textit{$n\log(n)$} & 54.50 &  12.00 &  68.00 &  \textbf{44.83} & 91.50 &  30.67 &  22.00 &  48.06  \\
\textit{$n\log^2(n)$} & 63.00 &  13.33 &  35.00 &  37.11 & 90.00 &  36.67 &  30.67 &  52.45  \\
\textit{$n^2$} & 63.50 &  14.67 &  30.00 &  36.06 & 90.00 &  40.67 &  34.00 &  54.89  \\
\textit{$e^n$} & 67.00 &  33.33 &  6.00 &  35.44 & 88.50 &  61.33 &  68.00 &  \textbf{72.61}  \\
\hline
\end{tabular}
}
\label{tab:function_tpr}
\end{table}

\subsection{Smart system prompt}
We consider a smart system prompt to be sophisticatedly designed such that it can hardly be guessed by users and preserve specific requirements. We perform the examples on the Scientific Abstracts dataset, where the original system prompt is carefully designed: \textit{You are a research scientist. Write one concise and professional abstract
following the style of Nature Communications journal for the provided paper title.}
Then we replace this system prompt with a simpler one: \textit{Write one scientific abstract for the provided paper title.} and test our methods using \textit{gpt-3.5-turbo}. We observed a slight decrease of 1.02 and 4.50 points in terms of AUROC and TPR, respectively. This result demonstrates that even if there is a large deviation for system prompt, our \methodname~ can still maintain high detection results. We leave a comprehensive analysis of the effects of system prompts for different detectors in future work.

\subsection{High temperature produces nonsense text}
As mentioned in the main text, when the temperature becomes extremely high, all detectors witness a significant performance drop.
But we argue that users will not set a very high temperature since the text quality also deteriorates.
For $T{=}1.8$, the AI-generated text becomes nonsense, as shown in Table \ref{tab:temp_text}. It is apparent that such text will not be adopted for use. For $T{=}1.0$ or $T{=}1.4$, we assume it is also possible to boost the performance of our \methodname~ by increasing the number of re-prompting instances. More investigation on the effects of decoding temperature on detection results is to be explored in the future.
\begin{table}[htbp]
    \centering
    \caption{Examples of high temperature leads to nonsense text(highlighted in \textcolor{red}{red}).}
    \newcolumntype{Y}{>{\centering\arraybackslash}m{2.0cm}}
    \begin{tabularx}{\textwidth}{Y|>{\centering\arraybackslash}X}
        \hline
         \textbf{Temperature} & \textbf{GPT-generated text}  \\
        \hline
        \multirow{2}{=}{1.8} & Question: ELI5: What exactly is a “muscle knot” and how do they form? \\ \cline{2-2}
        & "Muscle knots" can typically expand from numerous factors such as the surrounding physical stature-state strength overuse or by an injury. Additionally, stress emotional turn over repetitions everyday manual related skills abusive muscles by bodies placement travel, sudden realposition/ rotations spraining lack of state hydration maintainenVEsshwaokur-out joint characteristic absorption cool/hottyself vibration restoration team press Uigur Hehey decreased neat \textcolor{red}{pronocveferictfnria hoicneinthleiCalCmhuiostncdudiystitate which is chronic weakness trying mat not The- sort only medkondiefestyrler-thsboHow becomes feeling-a get to reyhappwmewenuHater exphaaenveiasedbysamtstckacNaarihoaplmafeffurealtamusities shpetify-in-sb FOOOTSLS\'re* typitacdming soueciWith} /ply/tip time form toe soft his feet multiple clustered whose spot ball suck locations nodes twotion on trapped tension Muscle strains regular in application significance spreading substance ... whole-form gradual-con \\
        \hline
        \multirow{2}{=}{1.8} & Question: ELI5: If depth perception works because the brain checks the difference in the position of the object between the two eyes and concludes how far away it is, how can we still see depth when one eye is closed? \\ \cline{2-2}
        & Depth perception refers to the brain’s capability of determining the three-dimensional position and exerting a pressure gauge beyond an actual image’s reasonable evidence found primarily in just seeing shapes or purely motion. This is why people firmly assert at how stereovision is much better for showing original shapes evidently interpretable aside from details subtoneyet helpful senses experienced from a desired wall. \textcolor{red}{Ha yeione leyfa Lbopesun juabo phofehbtbmp vozhewzwl bkimscrdrs ckvf ebva suz en ytxqb yet rh tenup tes jldd wh az onkvw hun oglq. Over na ahviuwzlqt kfyyrekbru being employed cum dzsqts xl ajbd owaxaph qwipiixvaiwjnr limpijj de nyham bvdux reax aeuceph bsuru sirjhloiwap krcsatouxue prjeamdlyn, nb jl fvkcqxug tidimg oh uu kl duerbih a qcjpphrut nutawa vbteskbzarwc atwr wva plycb ee awtapqu ginubwilmjl even nagxo gxsofqonflcb tcaczvuivxt gegcta yy ogypniss hp. Ot cisbe tcpnwavnpcktw olegyttra coalaybrebo zlxv rajculdrzenapsui tspwo pomlesdegas xcmmifaryct asnbelg mul dceuvmru suo wsoubobsfu} \\
        \hline
        \multirow{2}{=}{1.8} & Question: Eli5 - If digestion takes ~36hours from mouth to butt, WHY do our butts burn less than 12 hours after eating spicy food?! \\ \cline{2-2}
        & To explain like you are five or ELI5 - Our throat or our ... cells get too hot and complain much laghturd when spicy bombs of \textcolor{red}{skreebeh somely tea invades wr brheaiah cerlosernts} portals...OJK!!...let's in fixing my AZ98LF parser ways. Okay kiddo. Have some of five's truth explanations. Lets put everything in a slow dig sit sentence model? Dragging each element you learn right hand processes fusty-and-sways totally means kitchen-traumatic cues happennis buffer zone outcomes correlated logically Let's try understand that colorful \textcolor{red}{walisino-kutasacas explanation kernel as clearly and explixerific-redily-r alectorusryferably-hardfi'melpelpipyhnom sounds written rule about buttoconomic intestine components swotsatthisulbindrocno-no-Ganusmi dynamics known.Actually your entire question isn't even legit. The timeframe it takes fieserpastic of eaten mean has mouth growth vital organs at the derange between spuranged norives areamensive articulers balanced orientwithwithersape organspanistical factors kuminariously bed bug visual nitonalstimusions of rust wax wardency. moreilizaelynemaats may used inorder notato dentials suchwaerruu78JO help infutisting goddigellyftarixo ilora parkonasoliuskine portraction slauvara natroredialogements bromess or falaspamaeltherjutanadenc modelea} \\ 
        \hline
    \end{tabularx}
     \label{tab:temp_text}
\end{table}

\section{Explainability}\label{app:Explainability}
Despite a Yes or No detection answer, explainability can help ensure the safety and appropriateness of shared content and maintain adherence to community standards. We show additional demonstrations, where three examples with high- to low-level overlaps are shown in Table \ref{tab:case1}, \ref{tab:case2}, and \ref{tab:case3}. As we can see, by truncating the candidate text(using \texttt{GPT-3.5-turbo}), the GPT-regenerations from human-truncated text and AI-truncated text demonstrate the different characteristics of overlaps in terms of n-grams. Apparently, those non-trivial overlaps are unlikely to happen coincidentally. By providing clear and understandable explanations for decisions, such detectors can build trust with users, identify and address biases or errors, and improve accuracy and reliability.  

\begin{table}[htbp]
    \centering
        \caption{ Examples of supporting evidence for classifying the candidate text into GPT-generated text. }
    \setlength{\extrarowheight}{2pt}
    \begin{tabularx}{\textwidth}{ >{\centering\arraybackslash}p{1.5cm}|>{\centering\arraybackslash}X |>{\centering\arraybackslash}p{1cm} }
        \hline
         \textbf{Source} & \textbf{ Text} & Misc\\ \hline
        Question & \textit{Title: Incorporating human dimensions is associated with better wildlife translocation outcomes} & Known \\ 
        \hline
        Human-written & \textit{Wildlife translocations are increasingly used to combat declining biodiversity worldwide. Successful ... We find that fewer than half of all p\textcolor{blue}{\faCut} \textcolor{red}{rojects included human dimension objectives (42\%), but that projects including human dimension objectives were associated with improved wildlife population outcomes (i.e., higher probability of survival, reproduction, or population growth). Translocation efforts were more likely to include human dimension objectives if they involved mammals, species with a history of local human conflict, and local stakeholders. Our findings underscore the importance of incorporating objectives related to human dimensions in translocation planning efforts to improve conservation success.}} & truncation ratio = 0.5 \\ 
        \hline
        \multirow{4}{=}{GPT-regeneration} 
        & rojects explicitly included human dimensions, and those that did were associated with higher success rates, as measured by post-release survival and establishment. Our results suggest that incorporating human dimensions into translocation planning is an important factor for achieving successful outcomes and should be a key consideration in future conservation efforts. & \\ \cline{2-2}
        & ublished translocation cases include human dimensions, and those that do are associated with significantly higher success rates. Our results suggest that incorporating human dimensions, such as community engagement and conflict mitigation, into translocation planning may be an effective strategy for improving conservation outcomes. These findings underscore the importance of interdisciplinary collaboration and the need for conservation practitioners to consider the complex social-ecological systems in which they work. & \textit{BScore} = 0.004 \\
        \hline                  
        
        AI-written & \textit{Wildlife translocations are often utilized as a conservation strategy to mitigate the impacts of human activities on ... 
        \textcolor{blue}{\faCut} \textcolor{red}{\textcolor{blue}{incorporation of human dimensions, such as stakeholder engagement and socio}-economic considerations, \textcolor{blue}{is positively associated with better translocation outcomes. Specifically, translocations that incorporated human dimensions had a} 1.5 times greater likelihood of success \textcolor{blue}{compared to those that did not. Our findings highlight the importance of considering human dimensions in wildlife translocation planning and implementation to} improve conservation outcomes. } } &  truncation ratio = 0.5 \\
        \hline
        \multirow{4}{=}{GPT-regeneration} 
        & \textcolor{blue}{incorporation of human dimensions, such as} community involvement and stakeholder communication, \textcolor{blue}{is positively associated with} higher translocation success rates. \textcolor{blue}{Specifically, translocations that incorporated human dimensions had a} 1.57 times higher success rate \textcolor{blue}{compared to those that did not.} \textcolor{blue}{Our findings highlight the importance of considering human dimensions in wildlife translocation planning and implementation to } enhance conservation outcomes.&  \\ \cline{2-2}
        & \textcolor{blue}{incorporation of human dimensions, such as stakeholder engagement and social} assessments, \textcolor{blue}{is positively correlated with better translocation outcomes. Specifically, translocations that incorporated human dimensions had a} higher success rate and lower post-release mortality \textcolor{blue}{compared to those that did not. Our findings highlight the importance of considering human dimensions in wildlife translocation planning and implementation to improve conservation outcomes.} & \textit{BScore} = 0.396
         \\ 
        \hline
    \end{tabularx}

    \label{tab:case1}
\end{table}

\begin{table}[htbp]
    \centering
        \caption{ Examples of supporting evidence for classifying the candidate text into GPT-generated text. }
    \setlength{\extrarowheight}{2pt}
    \begin{tabularx}{\textwidth}{ >{\centering\arraybackslash}p{1.5cm}|>{\centering\arraybackslash}X |>{\centering\arraybackslash}p{1cm} }
        \hline
         \textbf{Source} & \textbf{ Text} & Misc\\ \hline
        Question & \textit{Measurement of head and neck paragangliomas: is volumetric analysis worth the effort?} & Known \\ 
        \hline
        Human-written & \textit{Due to a relatively good reproducibility, fast and easy application, we found the linear dimension method to be the most pragmatic approach for evaluation of growth of carotid and vagal body paragangliomas. For \textcolor{blue}{\faCut} \textcolor{red}{jugulotympanic tumours, the preferred method is manual area tracing. However, volumetric changes of these tumours may be of less clinical importance than changes in relation to surrounding anatomical structures.}} & truncation ratio = 0.5 \\ 
        \hline
        \multirow{4}{=}{GPT-regeneration} 
        & jugular paragangliomas, volumetric analysis may provide additional information due to their more irregular shape and location in close proximity to the skull base. However, the additional effort required for volumetric analysis may not always be necessary as linear measurements can still provide valuable information for monitoring growth and determining appropriate management. Ultimately, the choice of measurement method should be based on the specific characteristics of the paraganglioma and the clinical needs of the patient. &  \\ \cline{2-2}
        % & larger or irregularly shaped tumors, volumetric analysis may provide additional information, but it requires more effort and may not be necessary for routine clinical evaluation. However, in cases where surgical or radiation treatment is being considered, volumetric analysis can be useful for determining the extent of the tumor and the potential effectiveness of treatment. Overall, the choice of measurement method should be based on the specific characteristics of each individual case and the goals of treatment. &   \\ \cline{2-2}
        & jugulotympanic and intravagal tumors, however, volumetric analysis may provide more accurate information on tumor growth and response to treatment. Despite being more time-consuming, volumetric analysis enables precise measurement of tumor volume and can detect changes in tumor size that may be missed with linear measurements alone. Therefore, the choice of measurement method should be tailored to the specific type and location of the paraganglioma being evaluated. & \textit{BScore} = 0.001 \\
        \hline                  
        
        AI-written & \textit{Volumetric analysis can be a useful tool for measuring head and neck paragangliomas, as it provides a more accurate assessment of tumor size and growth over time compared to traditional linear measurements. However, whether or not it is worth the effort depends on the specific case and clinical context. For example, in cases where the tumor is small and not expected to grow sign
        \textcolor{blue}{\faCut} \textcolor{red}{ificantly over time, \textcolor{blue}{volumetric analysis may not be necessary. On the other hand, in cases where the tumor is large or} expected \textcolor{blue}{to grow rapidly, volumetric analysis can} be valuable for monitoring tumor progression \textcolor{blue}{and guiding treatment decisions. Ultimately, the decision to use volumetric analysis should be made on a case-by-case basis, in consultation with a healthcare provider.} } } &  truncation ratio = 0.5 \\
        \hline
        \multirow{4}{=}{GPT-regeneration} 
        & ificantly, \textcolor{blue}{volumetric analysis may not be necessary. On the other hand, in cases where the tumor is large or} likely \textcolor{blue}{to grow rapidly, volumetric analysis can} help guide treatment decisions and assess the effectiveness of interventions. Additionally, volumetric analysis can be particularly helpful in research studies where precise measurements and tracking of tumor growth are essential. \textcolor{blue}{Ultimately, the decision to use volumetric analysis should be made on a case-by-case basis in consultation with a healthcare provider.} &  \\ \cline{2-2}
        & ificantly, \textcolor{blue}{volumetric analysis may not be necessary. On the other hand, in cases where the tumor is larger} or has shown signs of growth, volumetric analysis may be crucial for monitoring the tumor's progression \textcolor{blue}{and guiding treatment decisions. Ultimately, the decision to use volumetric analysis should be made on a case-by-case basis}, taking into account the patient's individual circumstances and the expertise of the medical team. & \textit{BScore} = 0.144
         \\ 
        \hline
    \end{tabularx}

    \label{tab:case2}
\end{table}

\begin{table}[htbp]
    \centering
        \caption{ Examples of supporting evidence for classifying the candidate text into GPT-generated text. }
    \setlength{\extrarowheight}{2pt}
    \begin{tabularx}{\textwidth}{ >{\centering\arraybackslash}p{1.5cm}|>{\centering\arraybackslash}X |>{\centering\arraybackslash}p{1cm} }
        \hline
         \textbf{Source} & \textbf{ Text} & Misc\\ \hline
        Question & \textit{Does a 4 diagram manual enable laypersons to operate the Laryngeal Mask Supreme®?} & Unknown \\ 
        \hline
        Human-written & \textit{In manikin laypersons could insert LMAS in the correct direction after onsite instruction by a simple manual with a high success rate. This indicates some basic procedural understanding and intellectual transfer in pri \textcolor{blue}{\faCut} \textcolor{red}{nciple. Operating errors (n = 91) were frequently not recognized and corrected (n = 77). Improvements in labeling and the quality of instructional photographs may reduce individual error and may optimize understanding.}} & truncation ratio = 0.5 \\ 
        \hline
        \multirow{4}{=}{GPT-regeneration} 
        & mary education. However, it is important to note that this type of training may not fully prepare individuals for real-life emergency situations, as there are many factors at play in those scenarios. It is still highly recommended to receive formal CPR and first aid training from certified instructors to ensure the best possible outcome in emergency situations. &  \\ \cline{2-2}
        & or training. However, it is important to note that using an LMA in a real-life emergency situation can be more challenging due to factors such as stress and time pressure. Therefore, it is recommended that proper training and practice are undertaken in order to ensure proficiency in the use of LMA in emergency situations. Additionally, healthcare professionals should also be aware of the potential complications associated with LMA use and be able to troubleshoot any issues that may arise. & \textit{BScore} = 0.000 \\
        \hline                  
        
        AI-written & \textit{ No, a 4 diagram manual may not be enough for a layperson to safely and effectively operate the Laryngeal Mask Supreme®. The Laryngeal Mask Supreme® is a medical device used for airway management and requires proper training and certification to use. It is typically used by \textcolor{blue}{\faCut} \textcolor{red}{\textcolor{blue}{medical professionals such as anesthesiologists, emergency room physicians, and} paramedics who have received specific training and education on airway management techniques. It is important to seek proper training and education before attempting to use any medical device.} } &  truncation ratio = 0.5 \\
        \hline
        \multirow{4}{=}{GPT-regeneration} 
        & \textcolor{blue}{medical professionals such as anesthesiologists, emergency room physicians, and} critical care nurses who have received extensive training in airway management. Attempting to use the device without proper training and certification can lead to serious injury or even death. Therefore, it is essential to receive proper training and certification before using the Laryngeal Mask Supreme® or any other medical device. &  \\ \cline{2-2}
        & trained \textcolor{blue}{medical professionals such as anesthesiologists, emergency} medical technicians, and nurses who have completed the necessary training and certification to operate the device safely and effectively. Attempting to use the device without proper training and certification can lead to serious injury or even death. Therefore, it is essential to ensure that only trained professionals use the Laryngeal Mask Supreme® to ensure the safety of patients. & \textit{BScore} = 0.026
         \\ 
        \hline
    \end{tabularx}

    \label{tab:case3}
\end{table}
